# Supplementary material for: Fast Threshold Tests for Detecting Discrimination
Source: arXiv:1702.08536 ancillary file (2018-03-10)
Supplement: Supplementary file 1 [file supplementary_information.pdf]

# Fast Threshold Tests for Detecting Discrimination

## Supplementary Information

### 1 Proofs

**Proof of proposition 3.1** [Monotonicity] *Given a discriminant distribution  $\text{disc}(\phi, \mu_0, \sigma_0, \mu_1, \sigma_1)$ , the mapping  $g$  from signal space to probability space is monotonic if and only if  $\sigma_0 = \sigma_1$ .*

*Proof.* The mapping from signal space to probability space can be found with Bayes' rule:

$$\begin{aligned} g(x) = \Pr(Y = 1 \mid X = x) &= \frac{\Pr(Y = 1)N(x; \mu_1, \sigma_1)}{\Pr(Y = 1)N(x; \mu_1, \sigma_1) + \Pr(Y = 0)N(x; \mu_0, \sigma_0)} \\ &= \text{logit}^{-1}(Ax^2 + Bx + C) \end{aligned}$$

where

$$\begin{aligned} A &= \frac{\sigma_1^2 - \sigma_0^2}{2\sigma_0^2\sigma_1^2} & B &= \frac{\mu_1\sigma_0^2 - \mu_0\sigma_1^2}{\sigma_0^2\sigma_1^2} \\ C &= \frac{\sigma_1^2\mu_0^2 - \sigma_0^2\mu_1^2}{2\sigma_0^2\sigma_1^2} - \log\left(\frac{1-\phi}{\phi}\frac{\sigma_1}{\sigma_0}\right). \end{aligned}$$

This is the composition of a quadratic in  $x$  and the inverse logit function, which will be monotonic if and only if the quadratic is monotonic, requiring  $\sigma_0^2 - \sigma_1^2 = 0$ .  $\square$

**Proof of proposition 3.2** [2-parameter representation]: *Suppose  $\text{disc}(\phi, \mu_0, \sigma, \mu_1, \sigma)$  and  $\text{disc}(\phi', \mu'_0, \sigma', \mu'_1, \sigma')$  are two homoskedastic discriminant distributions. Let*

$$\delta = \frac{\mu_1 - \mu_0}{\sigma}$$

*and define  $\delta'$  analogously. Then the two distributions are identical if  $\phi = \phi'$  and  $\delta = \delta'$ . As a result, homoskedastic discriminant distributions can be parameterized by  $\phi$  and  $\delta$  alone.*

*Proof.* We establish this result by explicitly deriving the density of  $g(X)$ , where  $g$  is the usual mapping from signal to probability space. Doing so first requires computing the inverse transformation from probability space to signal space:

$$g^{-1}(p) = \frac{\mu_1^2 - \mu_0^2 - 2\sigma^2 \log\left(\frac{\phi}{1-\phi}\frac{1-p}{p}\right)}{2(\mu_1 - \mu_0)}.$$

Now,

$$\frac{d}{dp}(g^{-1}(p)) = \frac{\sigma^2}{p(1-p)(\mu_1 - \mu_0)}.$$

The density of  $X$  is

$$f_X(x) = \phi N(x; \mu_1, \sigma_1) + (1 - \phi)N(x; \mu_0, \sigma_0).$$

We can accordingly compute the density of  $g(X)$  by the change of variables formula:

$$\begin{aligned} f_P(p) &= f_X(g^{-1}(p)) \left| \frac{d}{dp}(g^{-1}(p)) \right| \\ &= \frac{\sigma}{\sqrt{2\pi p(1-p)}(\mu_1 - \mu_0)} \left[ \phi \exp \left( -\frac{\left( \alpha + \frac{(\mu_1 - \mu_0)^2}{\sigma^2} \right)^2}{8 \frac{(\mu_1 - \mu_0)^2}{\sigma^2}} \right) + (1 - \phi) \exp \left( -\frac{\left( \alpha - \frac{(\mu_1 - \mu_0)^2}{\sigma^2} \right)^2}{8 \frac{(\mu_1 - \mu_0)^2}{\sigma^2}} \right) \right], \end{aligned}$$

where

$$\alpha = 2 \log \left( \frac{\phi}{1 - \phi} \frac{1 - p}{p} \right).$$

Without loss of generality we can set  $\delta = (\mu_1 - \mu_0)/\sigma$ , resulting in a 2-parameter family of densities:

$$f_P(p) = \frac{1}{\sqrt{2\pi p(1-p)}\delta} \left[ \phi \exp \left( -\frac{(\alpha + \delta^2)^2}{8\delta^2} \right) + (1 - \phi) \exp \left( -\frac{(\alpha - \delta^2)^2}{8\delta^2} \right) \right]. \quad (1)$$

□

**Proof that discriminant distributions are a subset of logit-normal mixtures:** Discriminant distributions approximate logit-normal distributions particularly well because they in fact form a subset of logit-normal mixture distributions. To see this, consider the following rearrangement of the first component in the mixture in Eq. (1) (ie, the component with weight  $\phi$ ):

$$\frac{\exp \left( -\frac{(2 \log(\frac{\phi}{1-\phi} \frac{1-p}{p}) + \delta^2)^2}{8\delta^2} \right)}{\sqrt{2\pi p(1-p)}\delta} = \frac{\exp \left( -\frac{(\text{logit}(p) - (\text{logit}(\phi) + \frac{\delta^2}{2}))^2}{2\delta^2} \right)}{\sqrt{2\pi p(1-p)}\delta}.$$

This is the density of a logit-normal with parameters  $\mu = \text{logit}(\phi) + \frac{\delta^2}{2}$  and  $\sigma = \delta$ . Thus, we can express the discriminant distribution as a specific 2-parameter mixture of logit-normals (where  $f_l(x; \mu, \sigma)$  is the density function of the logit-normal):

$$f_P(p) = \phi f_l \left( p; \text{logit}(\phi) + \frac{\delta^2}{2}, \delta \right) + (1 - \phi) f_l \left( p; \text{logit}(\phi) - \frac{\delta^2}{2}, \delta \right).$$

In this form, we can see that for small  $\delta$  or  $\phi$  close to 0 or 1, the distribution is almost equivalent to a (single) logit-normal.

## 2 Supplementary figures

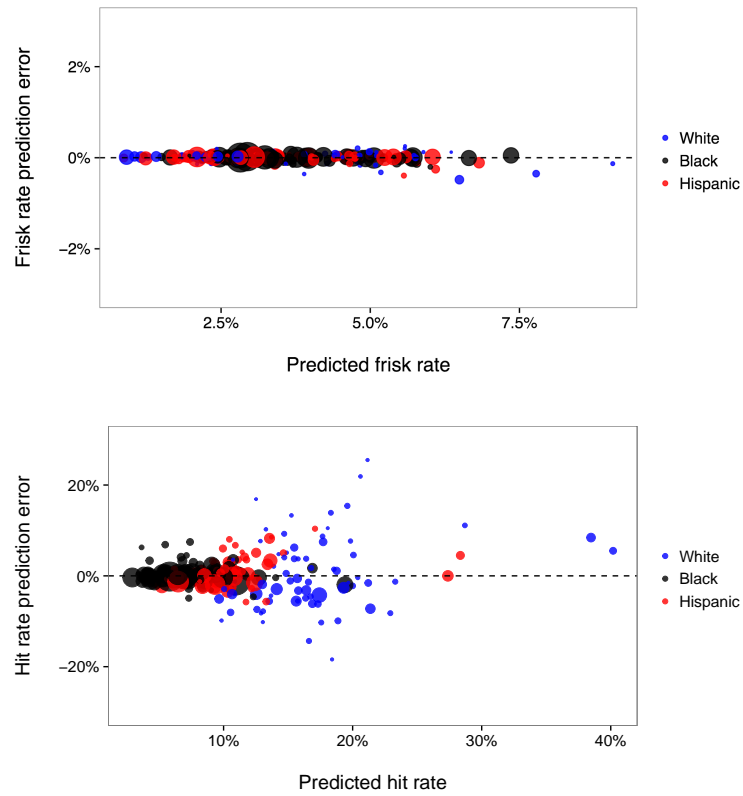

Figure 1: Posterior predictive checks for frisk rate and hit rate in stop-and-frisk data. Each point represents one precinct-race pair. Points are sized by the number of stops for that precinct and race.

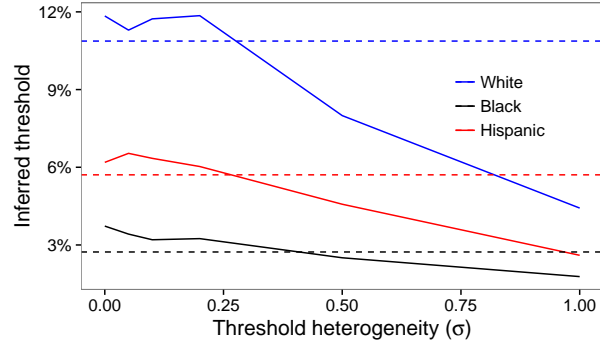

Figure 2: Inferred frisk thresholds when the model is fit to simulated data, where the threshold applied to each stop is perturbed by logit-normal noise. The dashed lines indicate the unperturbed thresholds. Racial disparities in thresholds persist even as large amounts of noise are introduced.

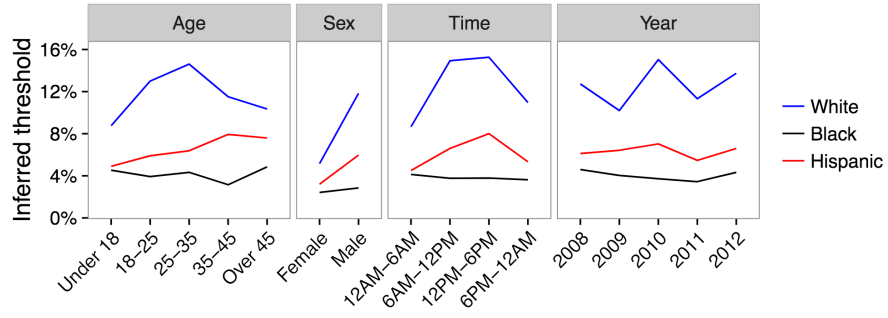

Figure 3: Frisk thresholds inferred on disaggregated subsets of the primary dataset. While thresholds vary across subsets, thresholds for whites are consistently higher than thresholds for blacks and Hispanics.

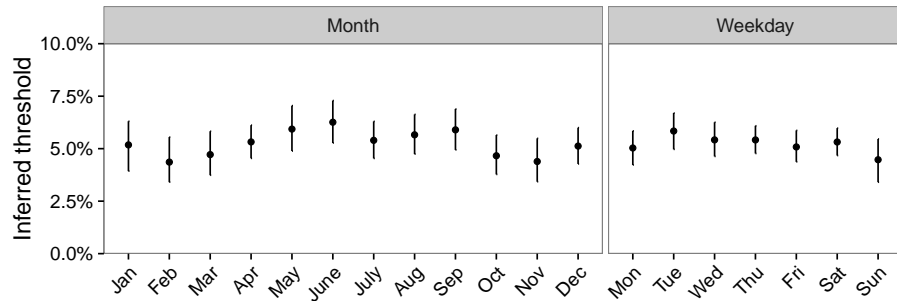

Figure 4: Placebo test: frisk thresholds inferred using month or weekday rather than race show only slight variation, as expected. Vertical lines denote 95% credible intervals.

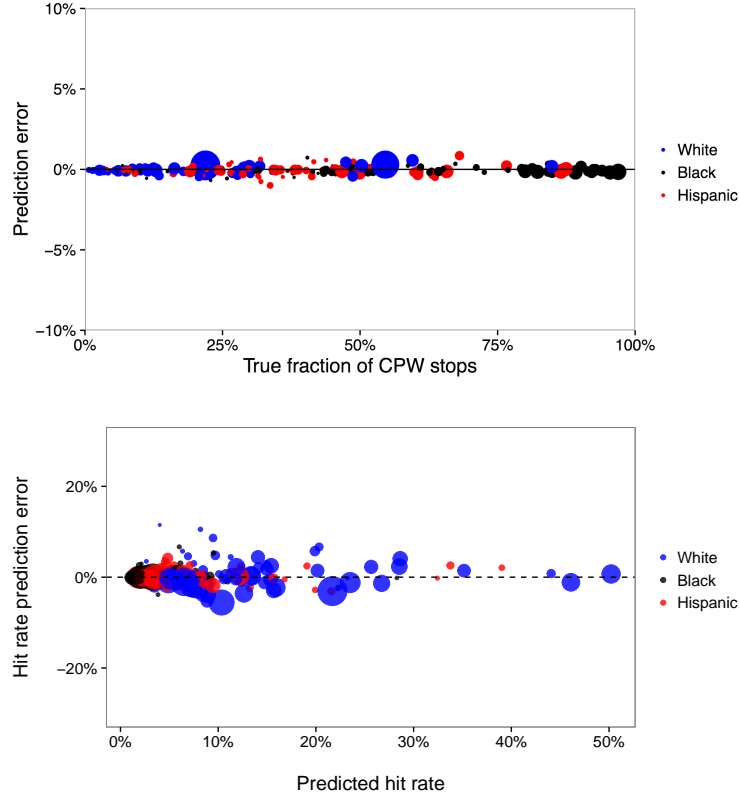

Figure 5: Posterior predictive checks for stop model. Each point represents one precinct-race pair. Points are sized by the population of each race in each precinct.

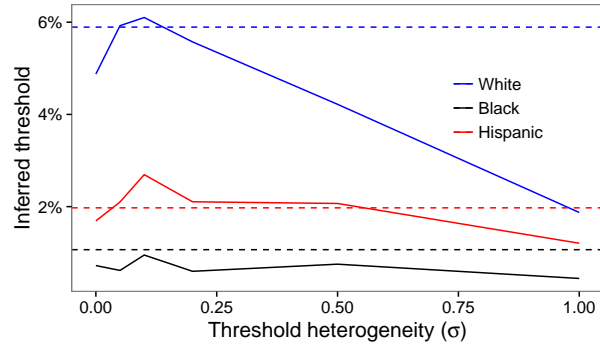

Figure 6: Inferred stop thresholds when the model is fit to simulated data, where the threshold applied to each stop is perturbed by logit-normal noise. The racial disparities in thresholds persist even as large amounts of noise are introduced.

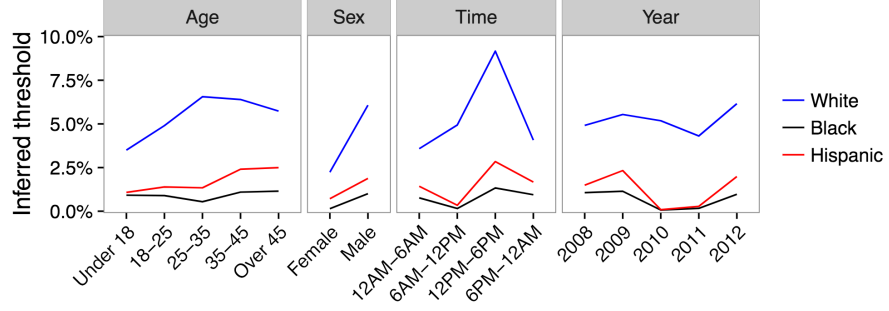

Figure 7: Stop thresholds inferred on disaggregated subsets of the primary dataset. While thresholds vary across subsets, thresholds for whites are consistently higher than thresholds for blacks and Hispanics.

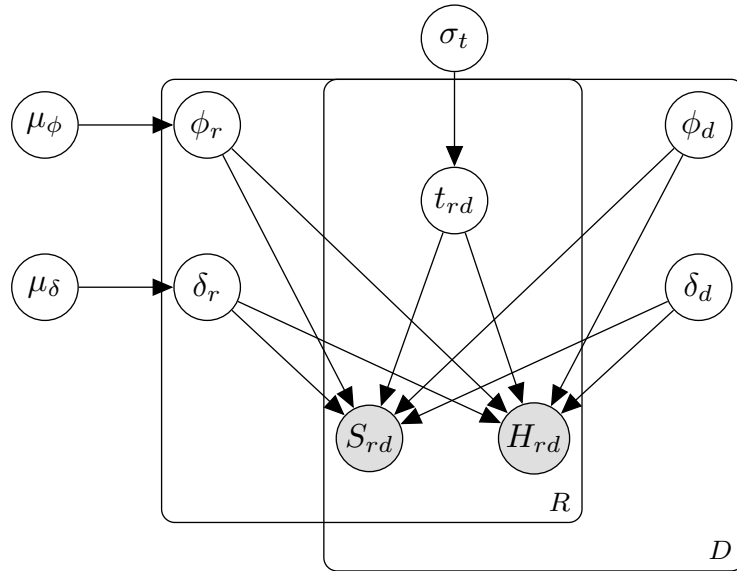

Figure 8: Graphical representation of the generative model for stop decisions. Observed outcomes are shaded, and unshaded nodes are latent variables inferred from data.
